# Supplementary material for: Power sector effects of alternative options for de-fossilizing heavy-duty vehicles -- go electric, and charge smartly
Source: arXiv:2303.16629 source file (2024-05-24)

Grid2Wheel    Grid2Bat    HDV discharging to the grid    Residual load (2<sup>nd</sup> axis)

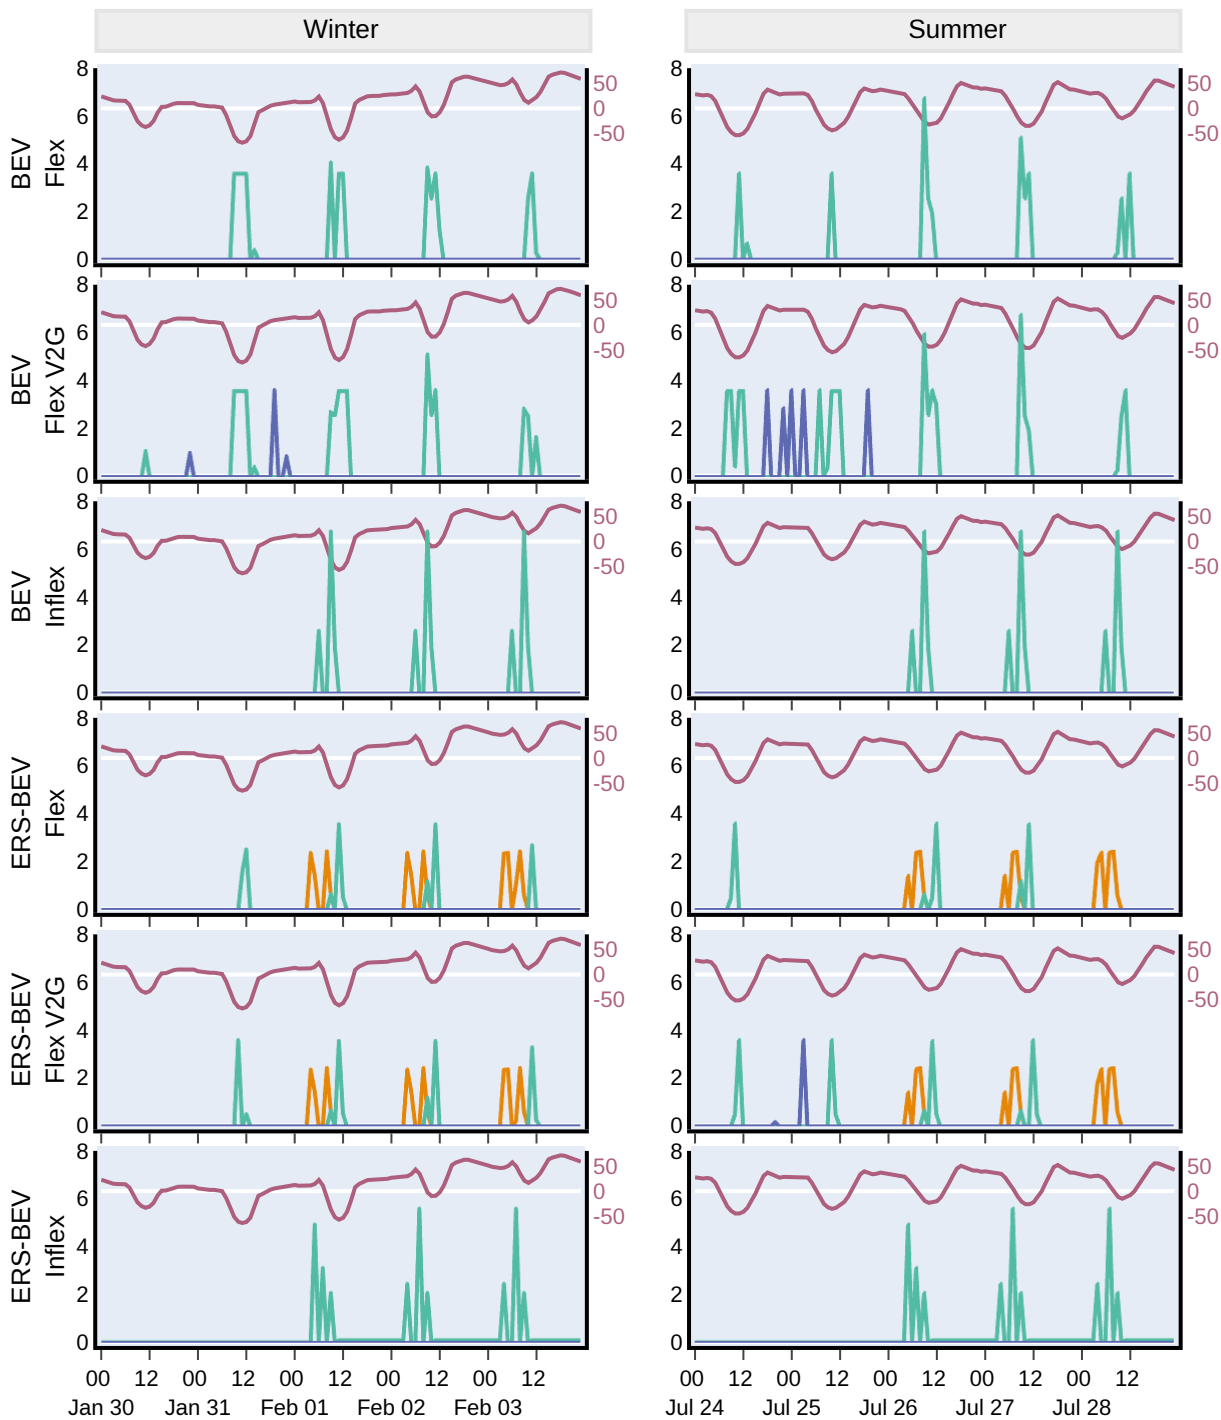

Supplement: Supplementary file 2 [file Fig_SI12.pdf]
