# Supplementary material for: Power sector effects of alternative options for de-fossilizing heavy-duty vehicles -- go electric, and charge smartly
Source: arXiv:2303.16629 source file (2024-05-24)

Germany + neighbors

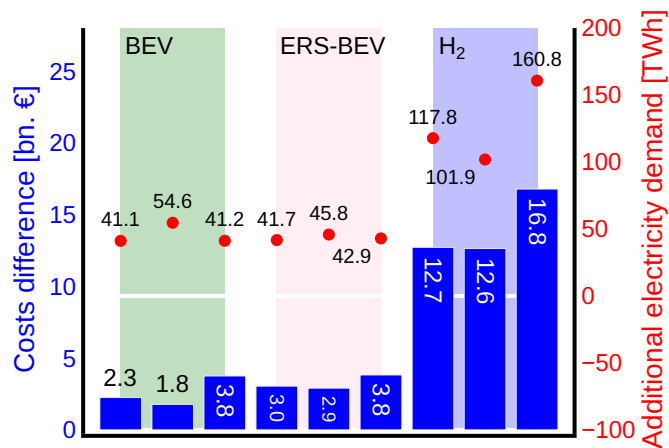

Germany only

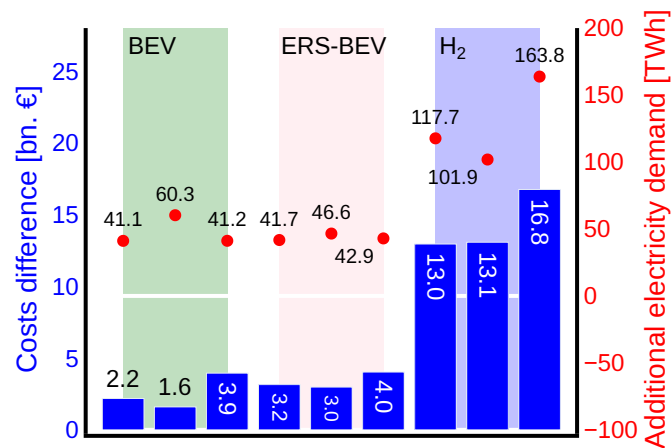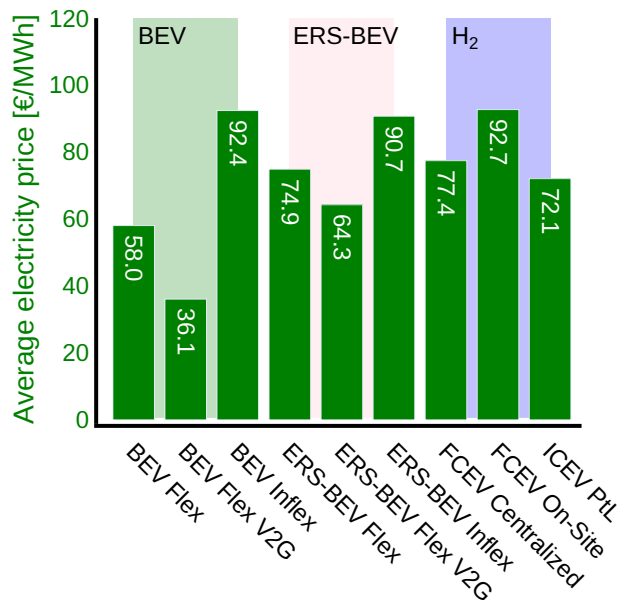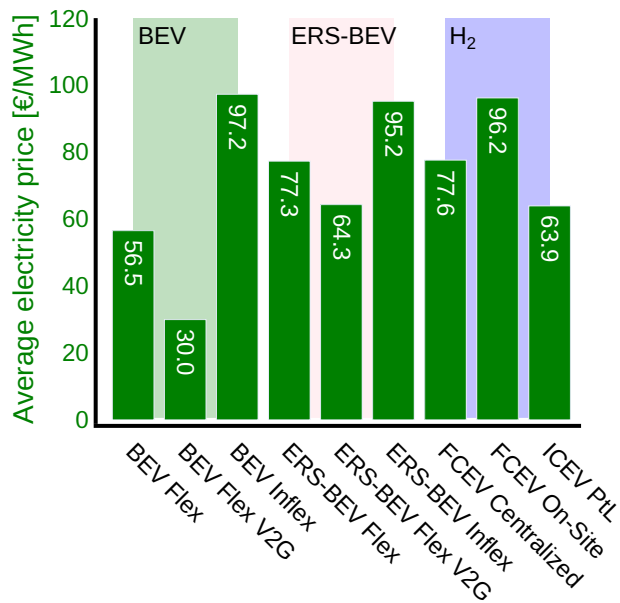

Supplement: Supplementary file 4 [file Fig_SI14.pdf]
