# Supplementary material for: Power sector effects of alternative options for de-fossilizing heavy-duty vehicles -- go electric, and charge smartly
Source: arXiv:2303.16629 source file (2024-05-24)

Without wind capacity constraint

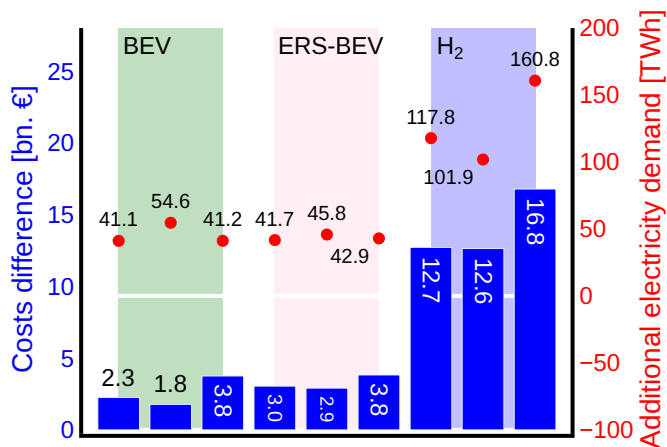

With wind capacity constraint

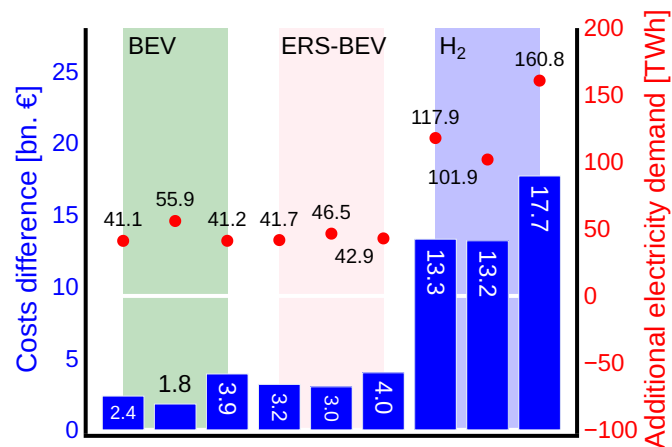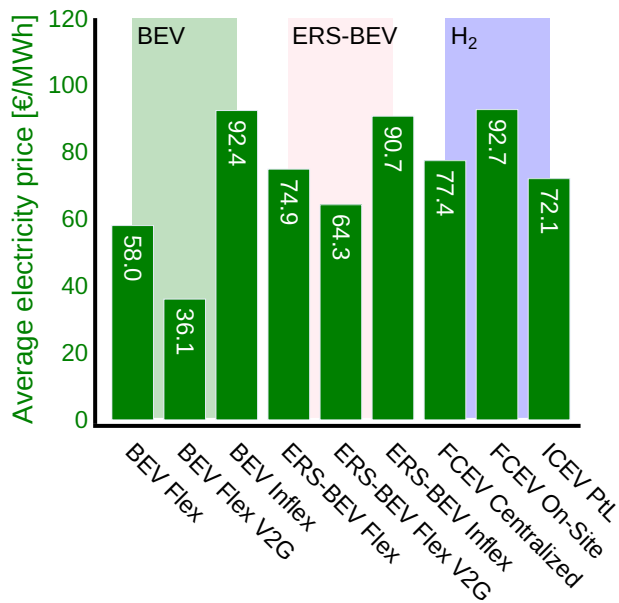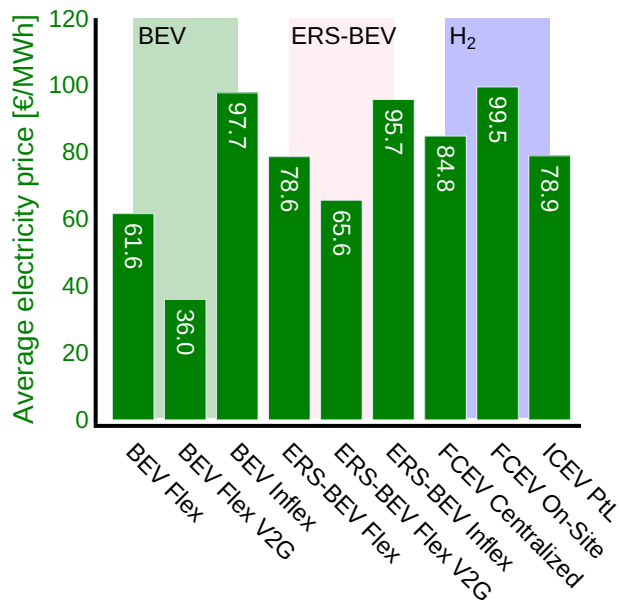

Supplement: Supplementary file 5 [file Fig_SI17.pdf]
